# Supplementary material for: Partially Observable RL with B-Stability: Unified Structural Condition and Sharp Sample-Efficient Algorithms
Source: arXiv:2209.14990 source file (2022-12-16)
Supplement: Supplementary file 1 [file valuelink.tex]

\section{Understanding the value link function}

The value link function for POMDPs is introduced in~\citep{uehara2022provably} to design model-free (value- and policy-based) algorithms for POMDPs. In this section we collect some properties of the value link function. 

\begin{definition}[Value link function]
A function $g^\pi_h:\cZ_{h-1}\times \cO\to\R$ is said to be a \emph{value link function} for policy $\pi$ at step $h\in[H]$ if
\begin{align*}
    \E\brac{ g^\pi_h(\tau_{h-1}, o_h) | \tau_{h-1}, s_h } = V^\pi_h(\tau_{h-1}, s_h) \quad \textrm{for all}~(\tau_{h-1}, s_h) \in \cZ_{h-1}\times \cS.
\end{align*}
In vector form, 
\begin{align*}
    \O_h^\top g^\pi_h(\tau_{h-1}, \cdot) = V^\pi_h(\tau_{h-1}, \cdot).
\end{align*}
\end{definition}

For undercomplete weakly-revealing POMDPs, the value link function exists by utilizing the pseudo-inverse of $\O_h$:
\begin{align*}
    g^\pi_h(\tau_{h-1}, \cdot) \defeq \O_h^{\dagger\top} V^\pi_h(\tau_{h-1}, \cdot).
\end{align*}
However, notice that the value link function is not unique. For example, take any other vector $\bu\in\R^O$ orthogonal to the column space $\O_h$ (that is, $\O_h^\top \bu=\bzero$). Then it is easy to see that
\begin{align*}
    \wt{g}^\pi_h(\tau_{h-1}, \cdot) \defeq \O_h^{\dagger\top} V^\pi_h(\tau_{h-1}, \cdot) + \bu
\end{align*}
is also a value link function for $\pi$.


\paragraph{Bellman equation}
The above invariance suggests that, for value link functions, we cannot hope for the Bellman equation to hold \emph{point-wise} for any $(\tau_{h-1}, o_h)$. Instead, we can only hope for the Bellman equation to hold over any distribution of $o_h$ induced by some state $s_h$. 

\begin{lemma}[Bellman equation for value link function]
\label{lemma:value-link-bellman}
Let $g^\pi=\{g^\pi_h\}_{h\in[H]}$ be a value link function for policy $\pi$. Then for any $h\in[H]$ and any $(\tau_{h-1}, s_h)\in\cZ_{h-1}\times \cS$~\yub{that is visitable?}, we have
\begin{align*}
    \E_{a_h\sim \pi}\brac{ g^\pi_h(\tau_{h-1}, o_h) - \paren{r_h + g^\pi_{h+1}(\tau_h, o_{h+1})} | \tau_{h-1}, s_h} = 0.
\end{align*}
As a corollary, for any roll-in policy $\pi^{\rm in}$, we have
\begin{align*}
    \E_{a_{1:h-1}\sim \pi^{\rm in}, a_h\sim \pi}\brac{ g^\pi_h(\tau_{h-1}, o_h) - \paren{r_h + g^\pi_{h+1}(\tau_h, o_{h+1})}} = 0.
\end{align*}
\end{lemma}
The later corollary has first appeared in~\citep[Section 3.2]{uehara2022provably}.
\begin{proof}
Fix any $(\tau_{h-1}, s_h)\in\cZ_{h-1}\times\cS$. We have
\begin{align*}
    & \quad \E\brac{ g^\pi_h(\tau_{h-1}, o_h) | \tau_{h-1}, s_h } = V^\pi_h(\tau_{h-1}, s_h) \\
    & = \E_{a_h\sim\pi}\brac{ r_h + V^\pi_{h+1}(\tau_h, s_{h+1}) | \tau_{h-1}, s_h  } \\
    & = \E_{a_h\sim\pi}\brac{ r_h + \E\brac{ g^\pi_{h+1}(\tau_h, o_{h+1}) | \tau_h, s_{h+1} } | \tau_{h-1}, s_h  } \\
    & \stackrel{(i)}{=} \E_{a_h\sim\pi}\brac{ r_h + g^\pi_{h+1}(\tau_h, o_{h+1}) | \tau_{h-1}, s_h  }.
\end{align*}
Above, (i) uses the tower property of conditional expectations, as the filtration up to $\tau_h, s_{h+1}$ is a refinement of the filtration up to $\tau_{h-1}, s_h$. This completes the proof of the first claim. The second claim then follows by taking expectation over $(\tau_{h-1}, s_h)\sim \pi^{\rm in}$.
\end{proof}


\paragraph{Performance difference}
Let $g=\{g^V_h,g^Q_h\}_{h=1}^H$ be a V/Q-type value link function satisfying the consistency condition
\begin{align*}
    g^V_h(\tau_{h-1}, o_h) = \max_{a_h\in\cA} g^Q_h(\tau_{h-1}, o_h, a_h) \quad \textrm{for all}~(h, \tau_{h-1}, o_h).
\end{align*}
Define greedy policy $\pi^g$ as $\pi^g_h(\cdot|\tau_{h-1}, o_h)\defeq \argmax_{a_h\in\cA} g^Q_h(\tau_{h-1}, o_h, a_h)$. 

By standard performance difference arguments and using Lemma~\ref{lemma:value-link-bellman}, we have the performance difference 
\begin{align*}
    & \quad \E_{o_1}\brac{g^V_1(o_1)} - V^{\pi^g} = \sum_{h=1}^H \sum_{\tau_{h-1}, o_h, a_h} d^{\pi_g}_h(\tau_{h-1}, o_h, a_h) \brac{ g^Q_h - r_h - \P_hg^V_{h+1} }(\tau_{h-1}, o_h, a_h) \\
    & = \sum_{h=1}^H \<d^{\pi_g}_h, g^Q_h - \cT_h g^V_{h+1}\>_{\tau_{h-1}, o_h, a_h}.
\end{align*}

\yub{Check the above holds for any $g=g^{\theta',\pi}$, $\pi_g=\pi$, when true model is $\theta^\star$.}

\yub{Can we let $\tau_{h-1}$ appear only in $t$ and not $k$?}


\subsection{Value-based algorithm for POMDPs}

Goal: Design an algorithm based on value link functions with sharp rates (similar to OMLE).

The algorithm likely needs to incorporate
\begin{enumerate}
    \item Some form of Eluder dimension argument in low dimension such as $S$ (even though algorithm itself may not be global optimism).
    \item Not directly do the performance decomposition to Bellman errors and apply Bellman rank argument (since then the Bellman rank will be high).
\end{enumerate}

\subsection{A crude idea: model-based + value-based}
\paragraph{Operator language} Alternatively to \cref{lemma:value-link-bellman}, in operator language, we have
\begin{align*}
&V^{\pi}(\tau_{h-1};s_{h})
=
\sum_{o,a} \O_h(o|s_h)\pi(a|\tau_{h-1},o)\left[ r_h(o,a)+\T_{h,a}(s_{h+1}|s_{h}) V^{\pi}(\tau_{h-1},o,a;s_{h+1})\right]\\
\Rightarrow
&V^{\pi}(\tau_{h-1};\cdot)=\O_h^\top \left[\sum_{a}\pi(a|\tau_{h-1},\cdot)r_h(\cdot,a)\right]+\sum_{o,a}\pi(a|\tau_{h-1},o) \diag(\O_h(o|\cdot))\T_{h,a}^\top V^{\pi}(\tau_{h-1},o,a;\cdot)
\end{align*}
Therefore, we have a canonical choice of $g^{\pi}$ that is defined recursively by
\begin{align*}
g^{\pi}(\tau_{h-1};\cdot)=\left[\sum_{a}\pi(a|\tau_{h-1},o) r_h(o,a)\right]_{o}+\sum_{o,a}\pi(a|\tau_{h-1},o) \B_h(o,a)^\top g^{\pi}(\tau_{h-1},o,a;\cdot).
\end{align*}
More generally, for a test functional $f(\cdot;\cdot):\cT^h\times \cO\to\R$ ($f$ can be alternatively viewed as a function $\cT^h\to\R^O$) and a model $\theta$, we can consider the operator $\cB^{\theta}_{h}$ defined by
$$
[\cB^{\theta}_{h}f](\tau_{h-1},\cdot):=\frac{1}{A}\sum_{o,a} \B_h(o,a;\theta)^\top f(\tau_{h-1},o,a;\cdot),
$$
and by \cref{lemma:value-link-bellman}, it holds that
\begin{align*}
    \cond{ [\cB^{\theta^\star}_{h}f](\tau_{h-1}, o_h) -  f(\tau_h, o_{h+1}) }{\tau_{h-1},s_h; a_h\sim\Unif(\cA)} = 0.
\end{align*}
\yub{By integration this also holds without conditioning on $s_h$}
Furthermore, it holds that
\begin{align*}
\MoveEqLeft
    \cond{ [\cB^{\theta}_{h}f](\tau_{h-1}, o_h) -  f(\tau_h, o_{h+1}) }{\tau_{h-1}; a_h\sim\Unif(\cA)} \\
    &=
    \iprod{\bd(\tau_{h-1})}{\left[\left(\cB^{\theta}_{h}-\cB^{\theta^\star}_{h}\right)f\right](\tau_{h-1}, \cdot)}\\
    &=\frac{1}{A}\sum_{o,a} \iprod{\left(\B_{h}(o,a;\theta)-\B_{h}(o,a)\right)\bd(\tau_{h-1})}{f(\tau_{h-1},o,a, \cdot)}
\end{align*}

\paragraph{Constraints} Then, we can introduce a discriminator $x:\cT^{h-1}\to\R$ and define the loss function $\ell$ (w.r.t. a tuple $\zeta=(\tau_{h-1},o_h,a_h,o_{h+1})$) as
$$
\ell_h(f,x,\theta;\zeta):=\left[\cB^{\theta}_{h}f(\tau_{h-1}, o_h)-f(\tau_h, o_{h+1}) \right]x(\tau_{h-1})-\frac{1}{2}x(\tau_{h-1})^2.
$$
\yub{This deals with the double sampling. Alternatively, may use completeness and Golf-like confidence sets?}

If $\tau_{h-1}$ comes from some $\mu\in\Delta(\cT^{h-1})$ and $a_h$ is taken at uniform, then
\begin{align*}
&\epct{ \ell(f,x,\theta;\zeta) }
=
\cond{ x(\tau_{h-1})\iprod{\bd(\tau_{h-1})}{ \left(\cB^{\theta}_{h}-\cB^{\theta^\star}_{h}\right)f(\tau_{h-1}, \cdot)}-\frac{1}{2}x(\tau_{h-1})^2 }{\tau_{h-1}\sim\mu}\\
\Rightarrow
\max_{x} &\epct{ \ell(f,x,\theta;\zeta) }
=\sum_{\tau_{h-1}} \mu(\tau_{h-1})\iprod{\bd(\tau_{h-1})}{ \left(\cB^{\theta}_{h}-\cB^{\theta^\star}_{h}\right)f(\tau_{h-1}, \cdot)}^2,
\end{align*}
and when $f=\O_{h+1}(\theta)^{\dagger\top}\tilde{f}$ where $\tilde{f}$ ranges over all possible $\cT^{h}\to\{-1,+1\}^S$ functions, it holds that
\begin{align*}
\max_{x,f} &\epct{ \ell(f,x,\theta;\zeta) }
=\sum_{\tau_{h-1}} \mu(\tau_{h-1})\left[ \frac{1}{A}\sum_{o,a}  \nrm{ \O_{h+1}(\theta)^{\dagger}\left(\B_h(o,a;\theta)-\B_h(o,a)\right)\bd(\tau_{h-1}) }_1 \right]^2.
\end{align*}
Here, the size of the function class of $x$ and $f$ can be reduced significantly, by taking them parameterized by $(\theta,\theta')\in\Theta\times\Theta$:
\begin{align*}
    \widetilde{\cF}_{h}&:=\bigg\{
        \tilde{f}(\tau_{h},\cdot)=\sign\left[ \O_{h+1}(\theta)^{\dagger}\left(\B_h(o,a;\theta)-\B_h(o,a;\theta')\right)\bd(\tau_{h-1};\theta') \right]
        \bigg|
        \theta,\theta'\in\Theta
    \bigg\},\\
    \cF_{h}(\theta)&:=\bigg\{
        f(\tau_{h},\cdot)= \O_{h+1}(\theta)^{\dagger\top}\tilde{f}(\tau_{h},\cdot)
        \bigg|
        \tilde{f}\in\widetilde{\cF}_{h}
    \bigg\},\\
    \cX_{h}(\theta)&:=\bigg\{
        x:\tau_{h}\mapsto  \iprod{\bd(\tau_{h-1};\theta')}{ \left(\cB^{\theta}_{h}-\cB^{\theta'}_{h}\right)\left(\O_{h+1}(\theta)^{\dagger\top}\tilde{f}(\tau_{h},\cdot)\right)}
        \bigg|
        \theta'\in\Theta, \tilde{f}\in\widetilde{\cF}_{h}
    \bigg\}.
\end{align*}
The above constructions work for at least the case $\Theta$ is a finite model class. When $\Theta$ is an infinite set, then perhaps we need to replace $\sign$ with a Lipschitz approximation.~\yub{Take $1/\eps$-Lipschitz version of sign?}

\begin{algorithm}[H]
	\caption{\textsc{A Naive Algorithm}} \begin{algorithmic}[1]\label{alg:naive}
   \STATE \textbf{Input:} Model class $\Theta$, test function class $(\cF_h)$, discriminator class $(\cX_h)$.
   \STATE \textbf{Initialize:} confidence set $\Theta^1=\Theta$.
    \FOR{$k=1,\ldots,K$}
	  \STATE $(\theta^k,\pi^k) = \argmax_{\hat\theta\in\Theta^k,\pi} V^\pi(\hat\theta)$
	  \FOR{$h\in[H]$}
	    \STATE execute policy $\pi^k_{1:h-1}\circ \Unif(\cA)$  to collect a trajectory $\zeta^{k,h}=(\tau_{h-1},o_h,a_h,o_{h+1})$
    	\STATE add $\zeta^{k,h}$ into $\cD_h$
	  \ENDFOR
	  \STATE update
	  \begin{equation*}
	  \Theta^{k+1} = \bigg\{\theta \in \Theta: \max_{x\in\cX_h(\theta)}\max_{f\in\cF_h(\theta)} \widehat{\cL}_{h}^{k+1}(f,x,\theta)\leq \beta,\ \forall h\in[H] \bigg\}.
	  \end{equation*}
	  \ENDFOR
   \end{algorithmic}
\end{algorithm}
Here at the end of step $k$, based on the dataset $\cD^k_h$, we can define 
$$
\widehat{\cL}_{h}^{k+1}(f,x,\theta)
:=
\sum_{\zeta\in\cD^{k}_h} \ell(f,x,\theta;\zeta).
$$


By applying \cref{prop:discri}, we have the following proposition.
\begin{proposition}\label{prop:MVB-confidence}
The following two statements hold \highprobdemo\ simultaneously.

(a) For any $h\in[H]$,  $f\in\cF_h(\theta^\star)$, $x\in\cX_h(\theta^\star)$, and $k\in[K]$, it holds that
$$
\widehat{\cL}_{h}^k(f,x,\theta^\star)\leq \beta:=\frac{1}{\sigma^2}\cdot\bigO{\log|\cF_h||\cX_h||\Theta|+\log(HAK/\delta)}.
$$
Hence $\theta^\star\in\Theta^k$ always.

(b) For any $(h,\theta)\in[H]\times\Theta$, it holds that
$$
\max_{x\in\cX_h(\theta), f\in\cF_h(\theta)}\sum_{t<k} \EE_t[\ell(f,x,\theta;\zeta^{t,h})]\leq 2\max_{x\in\cX_h(\theta), f\in\cF_h(\theta)}\widehat{\cL}_{h}^k(f,x,\theta)+\bigO{\beta},
$$
where $\EE_t[\cdot]$ is the conditional expectation taken w.r.t. all information at the beginning of step $t$.
\yub{Currently, the proof is not union bound over $(x, f)$. Rather, it takes max over $x$ explicitly first. See Proposition~\ref{prop:discri}(b).}
\end{proposition}

Fact (b) will directly imply that, for all $\theta\in\Theta^k$,
\begin{align*}
\MoveEqLeft
\sum_{t<k}\sum_{\tau_{h-1}} \PP^{\pi^t}(\tau_{h-1})\left[ \frac{1}{A}\sum_{o,a}  \nrm{ \O_{h+1}(\theta)^{\dagger}\left(\B_h(o,a;\theta)-\B_h(o,a)\right)\bd(\tau_{h-1}) }_1 \right]^2\\
&=
\max_{x\in\cX_h(\theta), f\in\cF_h(\theta)}\sum_{t<k} \EE_t[\ell(f,x,\theta;\zeta^{t,h})]
\leq \bigO{\beta}.
\end{align*}
This is exactly \eqref{eqn:err-condition}, and completes the proof.

\begin{proof}\label{prop:MVB-confidence}
Applying \cref{prop:discri} (a), we see that \highprobs{2}, for all $h\in[H]$ and $(k,f,x)\in[K]\times\cF_h(\theta^\star)\times\cX_h(\theta^\star)$, it holds that
\begin{align*}
    \widehat{\cL}_{h}^t(f,x,\theta^\star)
    \leqsim \left(\nrm{\cF_h}_{\infty}+ \nrm{\cX_h}_{\infty}\right)^2 \log\left( |\cF_h||\cX_h|HK/\delta \right).
\end{align*}
Applying \cref{prop:discri} (b), we see that \highprobs{2}, for all $(h,\theta)\in[H]\times\Theta$ and $(k,f)\in[K]\times\cF_h(\theta)$, 
\begin{align*}
    \sum_{t<k} \EE_t[\ell(f,\hat{x},\theta;\zeta^{t,h})]
    \leq 2\sum_{t<k} \ell(f,\hat{x},\theta;\zeta^{t,h})
    +\bigO{\frac{1}{\sigma^2} \log\left( |\cF_h||\Theta|HK/\delta \right)}.
\end{align*}
where $\hat{x}$ is the maximizer of LHS (in $\cX_h(\theta)$). Taking $\max_{ f\in\cF_h(\theta)}$ in the above inequality completes the proof.
\end{proof}

\begin{proposition}\label{prop:discri}
Given a sequence of random variables $U_1, V_1, \cdots, U_T, V_T$, we let $\Fil_t:=\sigma(U_1, V_1, \cdots, U_t, V_t)$. 
Suppose $f,g$ are bounded measurable functions with $\abs{f}\leq M_f, \abs{g}\leq M_g$, and we let 
$$
L^t:=2f(V_t)g(U_t)-g(U_t)^2.
$$

(a) Suppose that $\cond{f(V_t)}{\Fil_{t-1}, U_t}=0$. Then \highprobdemo,
\begin{align*}
\sum_{t=1}^T L^t
\leq 2(M_f+M_g)^2\log\frac{1}{\delta}.
\end{align*}```

(b) Suppose that $g(U_t)=\cond{f(V_t)}{\Fil_{t-1}, U_t}$. Then \highprobdemo,
\begin{align*}
\sum_{t=1}^T \cond{\cond{f(V_t)}{ U_t}^2}{\Fil_{t-1}}\leq 
2\sum_{t=1}^T L^t
+ 16M_f^2\log\frac{1}{\delta}.
\end{align*}
\end{proposition}

\begin{proof}
We denote $h(U_t):=\cond{f(V_t)}{\Fil_{t-1}, U_t}$ for simplicity. By a simple calculation,
\begin{align*}
    \cond{L^t}{\Fil_{t-1}, U_t}&=2h(U_t)g(U_t)-g(U_t)^2,\\
    \condV{L^t}{\Fil_{t-1}, U_t}&=g(U_t)^2\condV{f(V_t)}{\Fil_{t-1}, U_t}\leq  M_{f}^{2}g(U_t)^2.
\end{align*}

Hence, if $h=0$, then we have
\begin{align*}
    \condV{L^t}{\Fil_{t-1}, U_t}\leq  M_{f}^{2}\cond{-L^t}{\Fil_{t-1}, U_t}.
\end{align*}
Therefore, by Freedman's inequality, \highprobdemo,
\begin{align*}
\sum_{t=1}^T \left(L^t-\cond{L^t}{\Fil_{t-1}, U_t}\right)
\leq \lambda \sum_{t=1}^T \condV{L^t}{\Fil_{t-1}, U_t} + \frac{\log(1/\delta)}{\lambda},
\end{align*}
for any (fixed) $\lambda\in(0,\frac{1}{(M_f+M_g)^2})$. Then we can take $\lambda=\frac{1}{2(M_f+M_g)^2}$ to derive
\begin{align*}
\sum_{t=1}^T L^t
\leq (1-\lambda M_{f}^{2})\sum_{t=1}^T \cond{L^t}{\Fil_{t-1}, U_t} + \frac{\log(1/\delta)}{\lambda}\leq \frac{\log(1/\delta)}{\lambda}.
\end{align*}

On the other hand, if $g=h$,
then we have
\begin{align*}
    \condV{L^t}{\Fil_{t-1}, U_t}\leq  M_{f}^{2}\cond{L^t}{\Fil_{t-1}, U_t}.
\end{align*}
Similarly, by Freedman's inequality, \highprobdemo,
\begin{align*}
-\sum_{t=1}^T \left(L^t-\cond{L^t}{\Fil_{t-1}}\right)
\leq \lambda \sum_{t=1}^T \condV{L^t}{\Fil_{t-1}} + \frac{\log(1/\delta)}{\lambda},
\end{align*}
for any (fixed) $\lambda\in(0,\frac{1}{4M_f^2})$. We can take $\lambda=\frac{1}{8M_f^2}$ to derive
\begin{align*}
\sum_{t=1}^T \cond{L^t}{\Fil_{t-1}}
\leq \frac{1}{1-\lambda M_{f}^{2}}\sum_{t=1}^T L^t + \frac{\log(1/\delta)}{\lambda(1-\lambda M_{f}^{2})}\leq 2\sum_{t=1}^T L^t+\frac{2\log(1/\delta)}{\lambda}.
\end{align*}
\end{proof}
